# Supplementary material for: JITLine: A Simpler, Better, Faster, Finer-grained Just-In-Time Defect Prediction
Source: arXiv:2103.07068 source file (2021-03-16)
Supplement: Supplementary file 1 [file appendix.tex]

\begin{table}[t]
\caption{The commit-level software metrics for Just-In-Time Defect Prediction provided by McIntosh and Kamei~\cite{McIntosh2018}.}
\resizebox{\textwidth}{!}{%
\begin{tabular}{|l|l|l|}
\hline
\textbf{Category}                                & \textbf{Name}              & Description                                                                                          \\ \hline
\multirow{2}{*}{\textbf{Size}}                   & \textbf{LA}                & The number of lines added by a commit.                                                               \\ \cline{2-3} 
                                                 & \textbf{LD}                & The number of lines deleted by a commit.                                                             \\ \hline
\multirow{4}{*}{\textbf{Diffusion}}              & \textbf{NS}                & The number of modified subsystems.                                                                   \\ \cline{2-3} 
                                                 & \textbf{ND}                & The number of modified directories.                                                                  \\ \cline{2-3} 
                                                 & \textbf{NF}                & The number of modified files.                                                                        \\ \cline{2-3} 
                                                 & \textbf{Entropy}           & The spread of modified lines across changed files.                                                   \\ \hline
\multirow{3}{*}{\textbf{History}}                & \textbf{Unique changes}    & The number of prior changes to the modified files.                                                   \\ \cline{2-3} 
                                                 & \textbf{Developers}        & The number of developers who have changed the modified files in the past.                            \\ \cline{2-3} 
                                                 & \textbf{Age}               & The time interval between the last and current changes.                                              \\ \hline
\multirow{4}{*}{\textbf{Exp.}} & \textbf{Prior changes}     & The number of prior changes that an author has participated in.                                      \\ \cline{2-3} 
                                                 & \textbf{Recent changes}    & The number of prior changes that an author has participated in weighted by the age of the changes.   \\ \cline{2-3} 
                                                 & \textbf{Subsystem changes} & The number of prior changes to the modified subsystem(s) that an author has participated in.         \\ \cline{2-3} 
                                                 & \textbf{Awareness}         & The proportion of the prior changes to the modified subsystem(s) that an author has participated in. \\ \hline
\multirow{4}{*}{\textbf{Review}}                 & \textbf{Iterations}        & The number of times that a change was revised prior to integration.                                  \\ \cline{2-3} 
                                                 & \textbf{Reviewers}         & The number of reviewers who have voted on whether a change should be integrated or abandonded.       \\ \cline{2-3} 
                                                 & \textbf{Comments}          & The number of non-automated, non-owner comments posted during the review of a change.                \\ \cline{2-3} 
                                                 & \textbf{Review window}     & The length of time between the creation of a review request and its final approval for integration.  \\ \hline
\end{tabular}%
}
\end{table}
